# Supplementary material for: Analytical harmonic vibrational frequencies with VV10-containing density functionals: Theory, efficient implementation, and benchmark assessments
Source: arXiv:2208.14639 ancillary file (2023-04-02)
Supplement: Supplementary file 1 [file SI.pdf]

**Supporting Information:**

**Analytical harmonic vibrational frequencies with**

**VV10-containing density functionals:**

**Theory, efficient implementation, and**

**benchmark assessments.**

Jiashu Liang,<sup>†</sup> Xintian Feng,<sup>‡</sup> Xiao Liu,<sup>†</sup> and Martin Head-Gordon<sup>\*,†,¶</sup>

<sup>†</sup> *Kenneth S. Pitzer Center for Theoretical Chemistry, Department of Chemistry,  
University of California at Berkeley, Berkeley, CA 94720, USA*

<sup>‡</sup> *Q-Chem Inc., Pleasanton, CA 94588, USA*

<sup>¶</sup> *Chemical Sciences Division, Lawrence Berkeley National Laboratory, Berkeley, CA  
94720, USA*

E-mail: mhg@cchem.berkeley.edu

# Contents

|                                                                |            |
|----------------------------------------------------------------|------------|
| <b>1 Optimization problems and template calculation inputs</b> | <b>S-2</b> |
| <b>2 Supplemental figures for main paper</b>                   | <b>S-5</b> |

## **1 Optimization problems and template calculation inputs**

For most jobs, we employed a template Q-Chem input (see Listing 1) to calculate frequencies at best theoretical geometries (initial geometries) and optimized geometries. However, we encountered considerable difficulties in optimizing the geometries of molecules in the Noncovalent Set. A significant number of jobs led to one or more (typically but not always small) imaginary frequencies at the optimized geometries, which contradicts correct convergence to a local minimum. Additionally, a few jobs can not get converged in 100 optimization cycles.

To get optimization converged in 50 cycles and eliminate imaginary frequencies, we have attempted a variety of techniques for optimization. First, we tried to switch to the new optimization package “libopt3” in Q-Chem 6.0, employ a bigger quadrature grid for higher accuracy, recompute the exact hessian every three optimization cycles, and loosen the convergence thresholds (see Listing 2). The default setting can be seen in the Q-Chem manual. This resolved roughly half of the problematic jobs.

Second, we disabled the symmetry restriction, replaced default internal coordinates with Cartesian coordinates, and continued adjusting the convergence thresholds (see Listing 3). The results resolved roughly one-third of the remaining problematic jobs.

Third, we compared the present frequencies with those obtained from finite difference calculations. The differences were all within  $1\text{ cm}^{-1}$ , ruling out the possibility of numerical errors from functional quadrature. Therefore, we speculated that there might be no minimum

in the current point group symmetry for this combination of functional and molecule. We decided to add a small perturbation to the optimization geometry in the direction of the imaginary frequency. For linear molecules, we skipped this step to keep the number of frequencies unchanged. Finally, a few jobs still had remaining imaginary frequencies after being perturbed three times and we just accepted their values.

**Listing 1:** Default Q-Chem input file

```
$molecule
0 1
{Molecule Coordinates}
$end

$rem
JOBTYPE freq
METHOD {METHOD}
BASIS {BASIS}
XC_GRID 000099000590
NL_GRID 1
THRESH 14
SCF_CONVERGENCE 9
SYMMETRY FALSE
MEM_TOTAL {MEMORY}
$end

@@@
$molecule
read
$end

$rem
JOBTYPE opt
METHOD {METHOD}
BASIS {BASIS}
XC_GRID 000099000590
NL_GRID 1
THRESH 14
SCF_CONVERGENCE 9
SYMMETRY FALSE
MEM_TOTAL {MEMORY}
SCF_GUESS read
GEOM_OPT_HESSIAN read
GEOM_OPT_TOL_GRADIENT 30
GEOM_OPT_TOL_DISPLACEMENT 500
GEOM_OPT_TOL_ENERGY 1
$end

@@@
$molecule
read
$end
```

```

$rem
JOBTYPE freq
METHOD {METHOD}
BASIS {BASIS}
XC_GRID 000099000590
NL_GRID 1
THRESH 14
SCF_CONVERGENCE 9
SYMMETRY FALSE
MEM_TOTAL {MEMORY}
SCF_GUESS read
$end

```

**Listing 2:** First try to get optimization converged in 50 cycles and eliminate imaginary frequencies

```

$molecule
0 1
{Molecule Coordinates}
$end

$rem
JOBTYPE opt
METHOD {METHOD}
BASIS {BASIS}
XC_GRID 000200000590
NL_GRID 1
THRESH 14
SCF_CONVERGENCE 10
SYMMETRY FALSE
MEM_TOTAL {MEMORY}
$end

$geom_opt
initial_hessian = exact
recompute_hessian = recompute
recompute_hessian_cycles = 3
hessian_verify = recomputed
final_vibrational_analysis = true
THRESH = 3e-4
DISPLACEMENT_CONVERGENCE = 1e-3
ENERGY_CONVERGENCE = 1e-6
MAX_DISPLACEMENT 4e-2
$end

```

**Listing 3:** Second try to eliminate imaginary frequencies

```

$rem
SYMMETRY FALSE
SYM_IGNORE TRUE
GEOM_OPT_SYMFLAG FALSE
JOBTYPE opt
METHOD {METHOD}

```

```
BASIS {BASIS}  
XC_GRID 000200000590  
NL_GRID 1  
THRESH 14  
SCF_CONVERGENCE 10  
MEM_TOTAL {MEMORY}  
$end
```

```
$geom_opt  
MAXITER 100  
COORDINATES Cartesian  
initial_hessian = exact  
recompute_hessian = recompute  
recompute_hessian_cycles = 5  
hessian_verify = recomputed  
final_vibrational_analysis = true  
THRESH = 3e-5  
DISPLACEMENT_CONVERGENCE = 1e-3  
ENERGY_CONVERGENCE = 3e-8  
MAX_DISPLACEMENT 8e-2  
$end
```

## 2 Supplemental figures for main paper

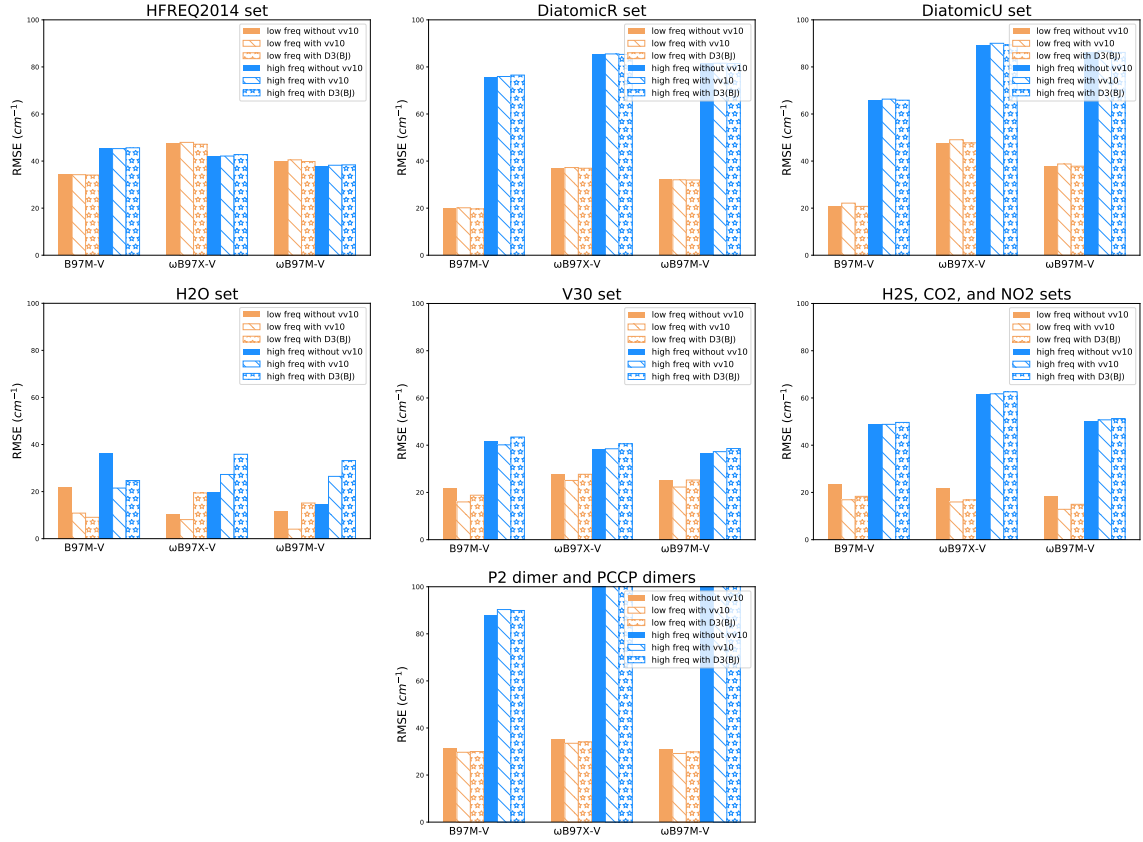

**Figure S1:** Comparison of the root-mean-squared errors (RMSEs) ( $\text{cm}^{-1}$ ) of low frequencies ( $< 1000 \text{ cm}^{-1}$ ) and high frequencies ( $\geq 1000 \text{ cm}^{-1}$ ) of B97M-V,  $\omega$ B97X-V, and  $\omega$ B97M-V with VV10, without VV10, and with D3(BJ) [replacing VV10 with D3(BJ)] at the optimized geometries (OptGs) on all subsets. The basis sets for each subset are the same as those in Figure 5.

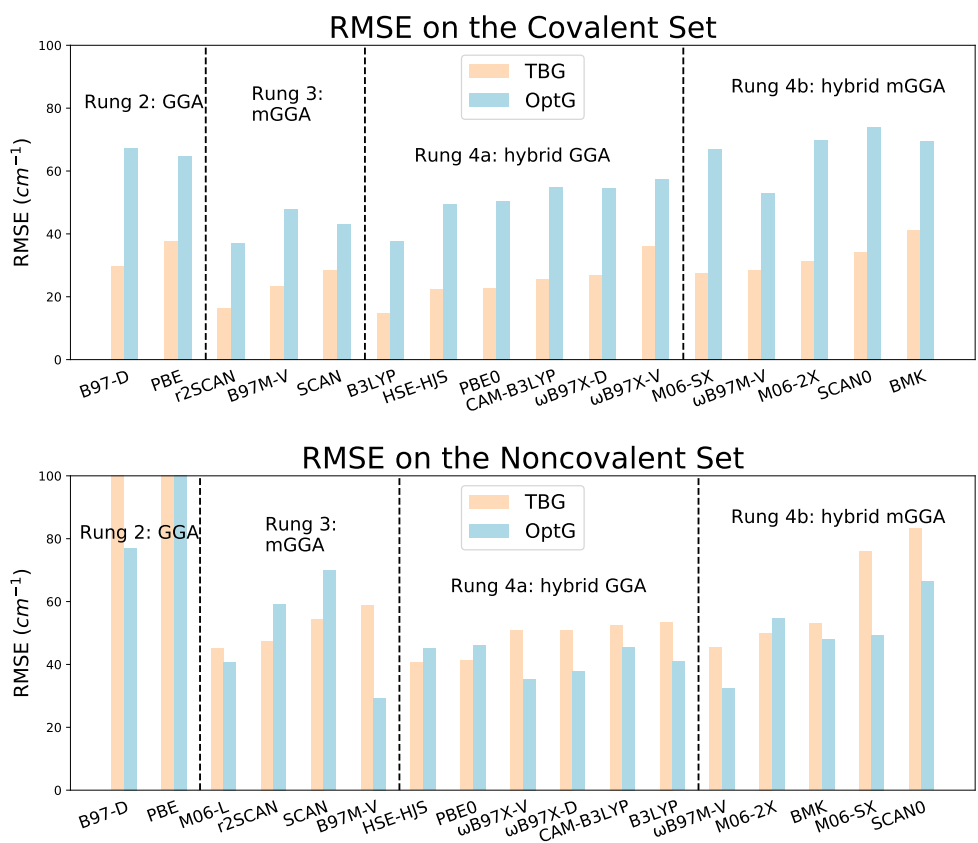

**Figure S2:** Comparison of the RMSEs ( $\text{cm}^{-1}$ ) of different functionals relative to TBEs using TBGs and optimized geometries (OptGs) on the Covalent Set and Noncovalent Set. The results are organized left to right in order of increasing RMSE using TBGs, on each rung of Jacob's Ladder. The D3(BJ) empirical correction is added to any functional without its own dispersion component. The basis sets used are the same as those in Figure 4.

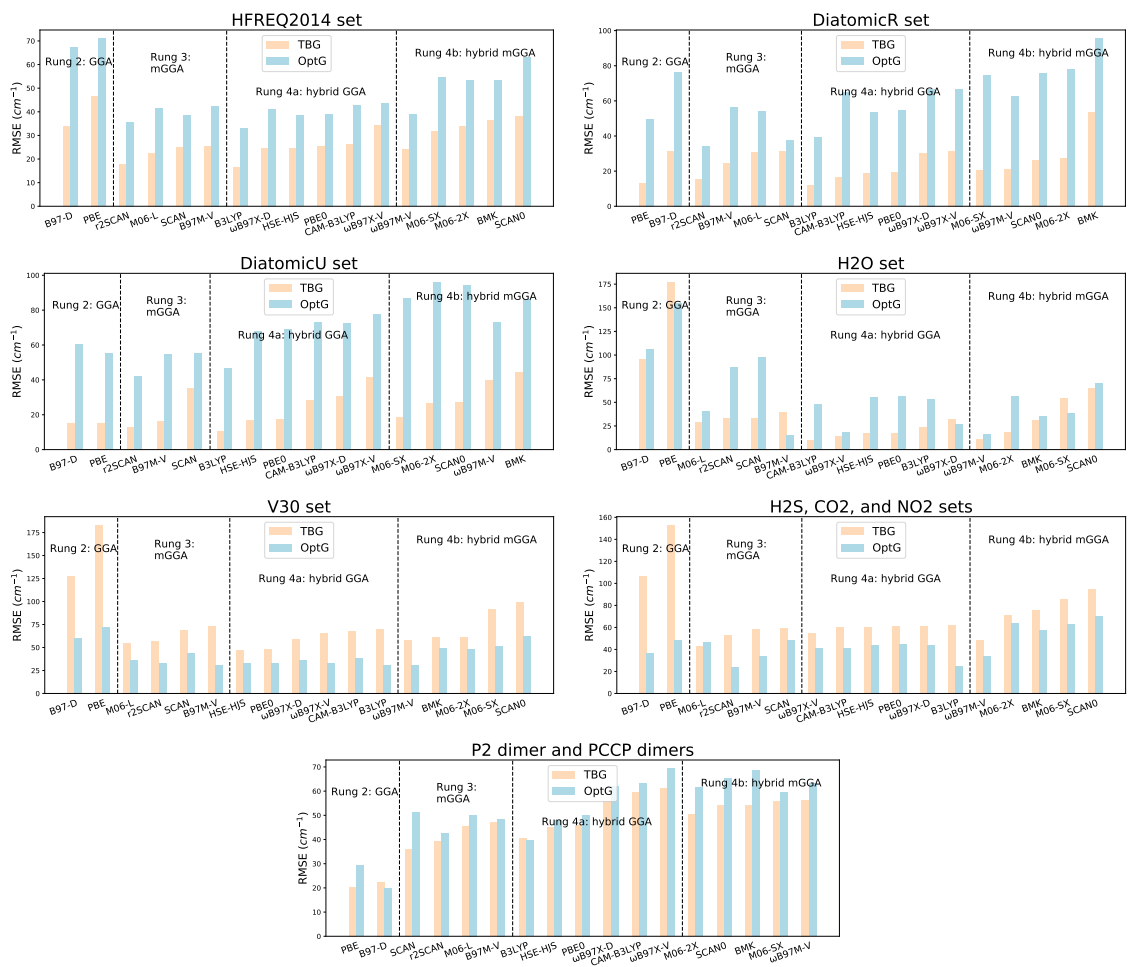

**Figure S3:** Comparison of the RMSEs ( $\text{cm}^{-1}$ ) of different functionals relative to TBEs using TBGs and optimized geometries (OptGs) on all subsets. The results are organized left to right in order of increasing RMSE using TBGs, on each rung of Jacob's Ladder. The basis sets used are the same as those in Figure 4.

| Molecule  | V30 classification | r2SCAN | B97M-V | B3LYP | $\omega$ B97X-V | $\omega$ B97M-V |
|-----------|--------------------|--------|--------|-------|-----------------|-----------------|
| C2H2_Ar   | nonpolar-nonpolar  | 23.54  | 49.82  | 33.97 | 57.24           | 50.45           |
| C2H2_C2H2 | nonpolar-nonpolar  | 22.92  | 49.25  | 34.18 | 56.56           | 49.65           |
| C2H4_Ar   | nonpolar-nonpolar  | 15.59  | 23.38  | 15.77 | 22.04           | 18.05           |
| N2_Ar     | nonpolar-nonpolar  | 43.40  | 62.46  | 55.21 | 78.17           | 76.66           |
| CH4_Ar    | nonpolar-nonpolar  | 11.62  | 20.92  | 12.22 | 8.46            | 15.04           |
| CH4_CH4   | nonpolar-nonpolar  | 14.85  | 20.02  | 11.89 | 8.06            | 15.80           |
| CH4_N2    | nonpolar-nonpolar  | 21.54  | 33.46  | 26.98 | 35.89           | 36.79           |
| CO2_Ar    | nonpolar-nonpolar  | 13.38  | 28.84  | 12.30 | 25.94           | 21.96           |
| CO2_CO2   | nonpolar-nonpolar  | 13.55  | 28.96  | 12.63 | 25.98           | 21.50           |
| CO2_N2    | nonpolar-nonpolar  | 26.50  | 41.96  | 28.35 | 44.90           | 42.00           |
| CO_Ar     | nonpolar-nonpolar  | 21.35  | 37.30  | 31.82 | 46.26           | 46.81           |
| CO_CO     | nonpolar-nonpolar  | 21.81  | 37.72  | 32.92 | 46.28           | 46.82           |
| N2_N2     | nonpolar-nonpolar  | 43.15  | 62.51  | 55.24 | 78.08           | 76.72           |
| H2O_Ar    | polar-nonpolar     | 19.20  | 20.91  | 19.44 | 18.38           | 10.18           |
| H2O_CH4   | polar-nonpolar     | 15.67  | 21.11  | 14.45 | 11.73           | 12.21           |
| H2O_CO2   | polar-nonpolar     | 19.71  | 26.51  | 19.76 | 23.48           | 20.80           |
| HF_N2     | polar-nonpolar     | 41.23  | 41.68  | 51.21 | 52.13           | 53.02           |
| NH3_Ar    | polar-nonpolar     | 7.97   | 28.21  | 12.43 | 21.65           | 17.52           |
| HF_Ar     | polar-nonpolar     | 32.27  | 7.88   | 37.83 | 12.80           | 21.08           |
| HF_C2H2   | polar-nonpolar     | 49.51  | 44.02  | 46.76 | 51.46           | 46.74           |
| HF_CH4    | polar-nonpolar     | 26.68  | 19.59  | 26.50 | 9.87            | 15.94           |
| HF_CO     | polar-nonpolar     | 26.53  | 23.58  | 33.99 | 30.95           | 33.43           |
| HF_H2O    | polar-polar        | 71.75  | 16.59  | 53.15 | 26.97           | 24.42           |
| HF_HCN    | polar-polar        | 49.39  | 42.58  | 49.99 | 46.41           | 43.61           |
| HF_HF     | polar-polar        | 53.04  | 10.57  | 51.62 | 17.59           | 26.98           |
| HF_NH3    | polar-polar        | 89.14  | 25.92  | 55.76 | 33.55           | 22.60           |
| NH3_NH3   | polar-polar        | 10.70  | 27.60  | 15.71 | 19.91           | 21.23           |
| CH3OH_H2O | polar-polar        | 29.46  | 14.11  | 22.37 | 10.04           | 8.79            |
| H2O_H2O   | polar-polar        | 29.74  | 18.67  | 26.19 | 13.26           | 9.54            |
| H2O_NH3   | polar-polar        | 29.62  | 26.17  | 23.57 | 17.13           | 15.03           |

**Figure S4:** Comparison of the RMSEs ( $\text{cm}^{-1}$ ) of r2SCAN-D3(BJ), B97M-V, B3LYP-D3(BJ),  $\omega$ B97X-V, and  $\omega$ B97M-V relative to TBEs using optimized geometries and the def2-QZVPP basis set on different molecule complexes of the V30 Set. D3(BJ) is omitted from the headings and henceforth for simplicity. Red fill indicates that the RMSEs of any of  $\omega$ B97X(M)-V or B97M-V are larger than those of B3LYP or r2SCAN, respectively. Green fill indicates that the RMSEs of VV10-containing functionals are smaller. It is evident that the VV10-containing functionals generally outperform r2SCAN and B3LYP for the polar-polar interactions, and slightly for the nonpolar-polar interactions. Interestingly, the VV10-containing functionals are systematically poorer for the nonpolar-nonpolar interactions.
